# Supplementary material for: ALT: Boosting Deep Learning Performance by Breaking the Wall between Graph and Operator Level Optimizations
Source: arXiv:2210.12415 source file (2022-10-29)
Supplement: Supplementary file 1 [file appendix.tex]

\newpage
\section{Appendix}
\begin{figure*}
\centering
\subfigure[C2D on Intel CPU]{\label{fig:motiv_C2D_llvm}{\includegraphics[width=0.32\textwidth]{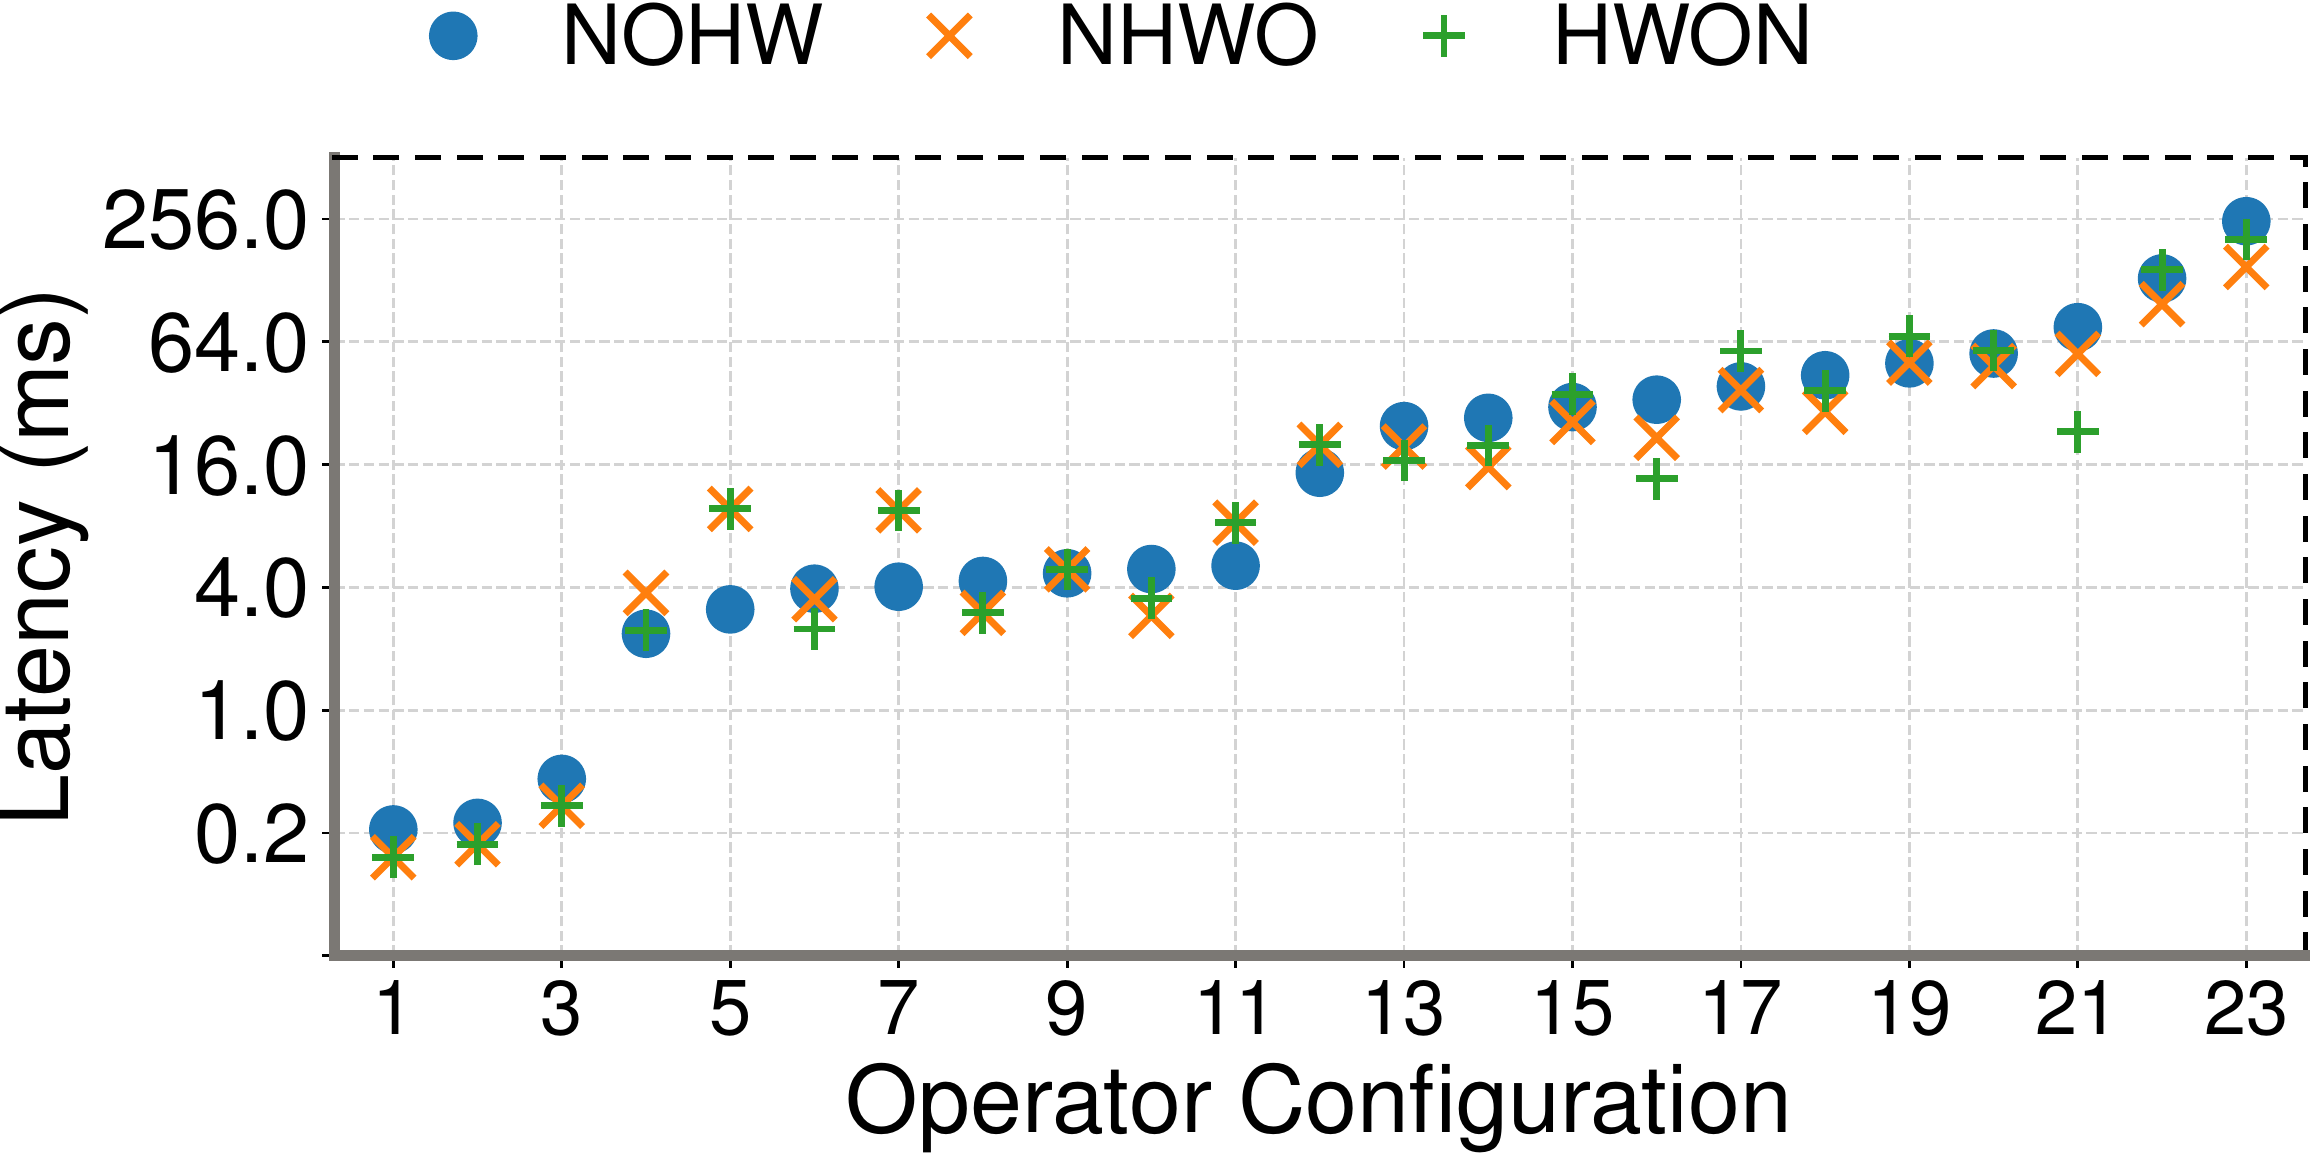}}}\hfill
~
\subfigure[C2D on NVIDIA GPU.]{\label{fig:motiv_C2D_cuda}{\includegraphics[width=0.32\textwidth]{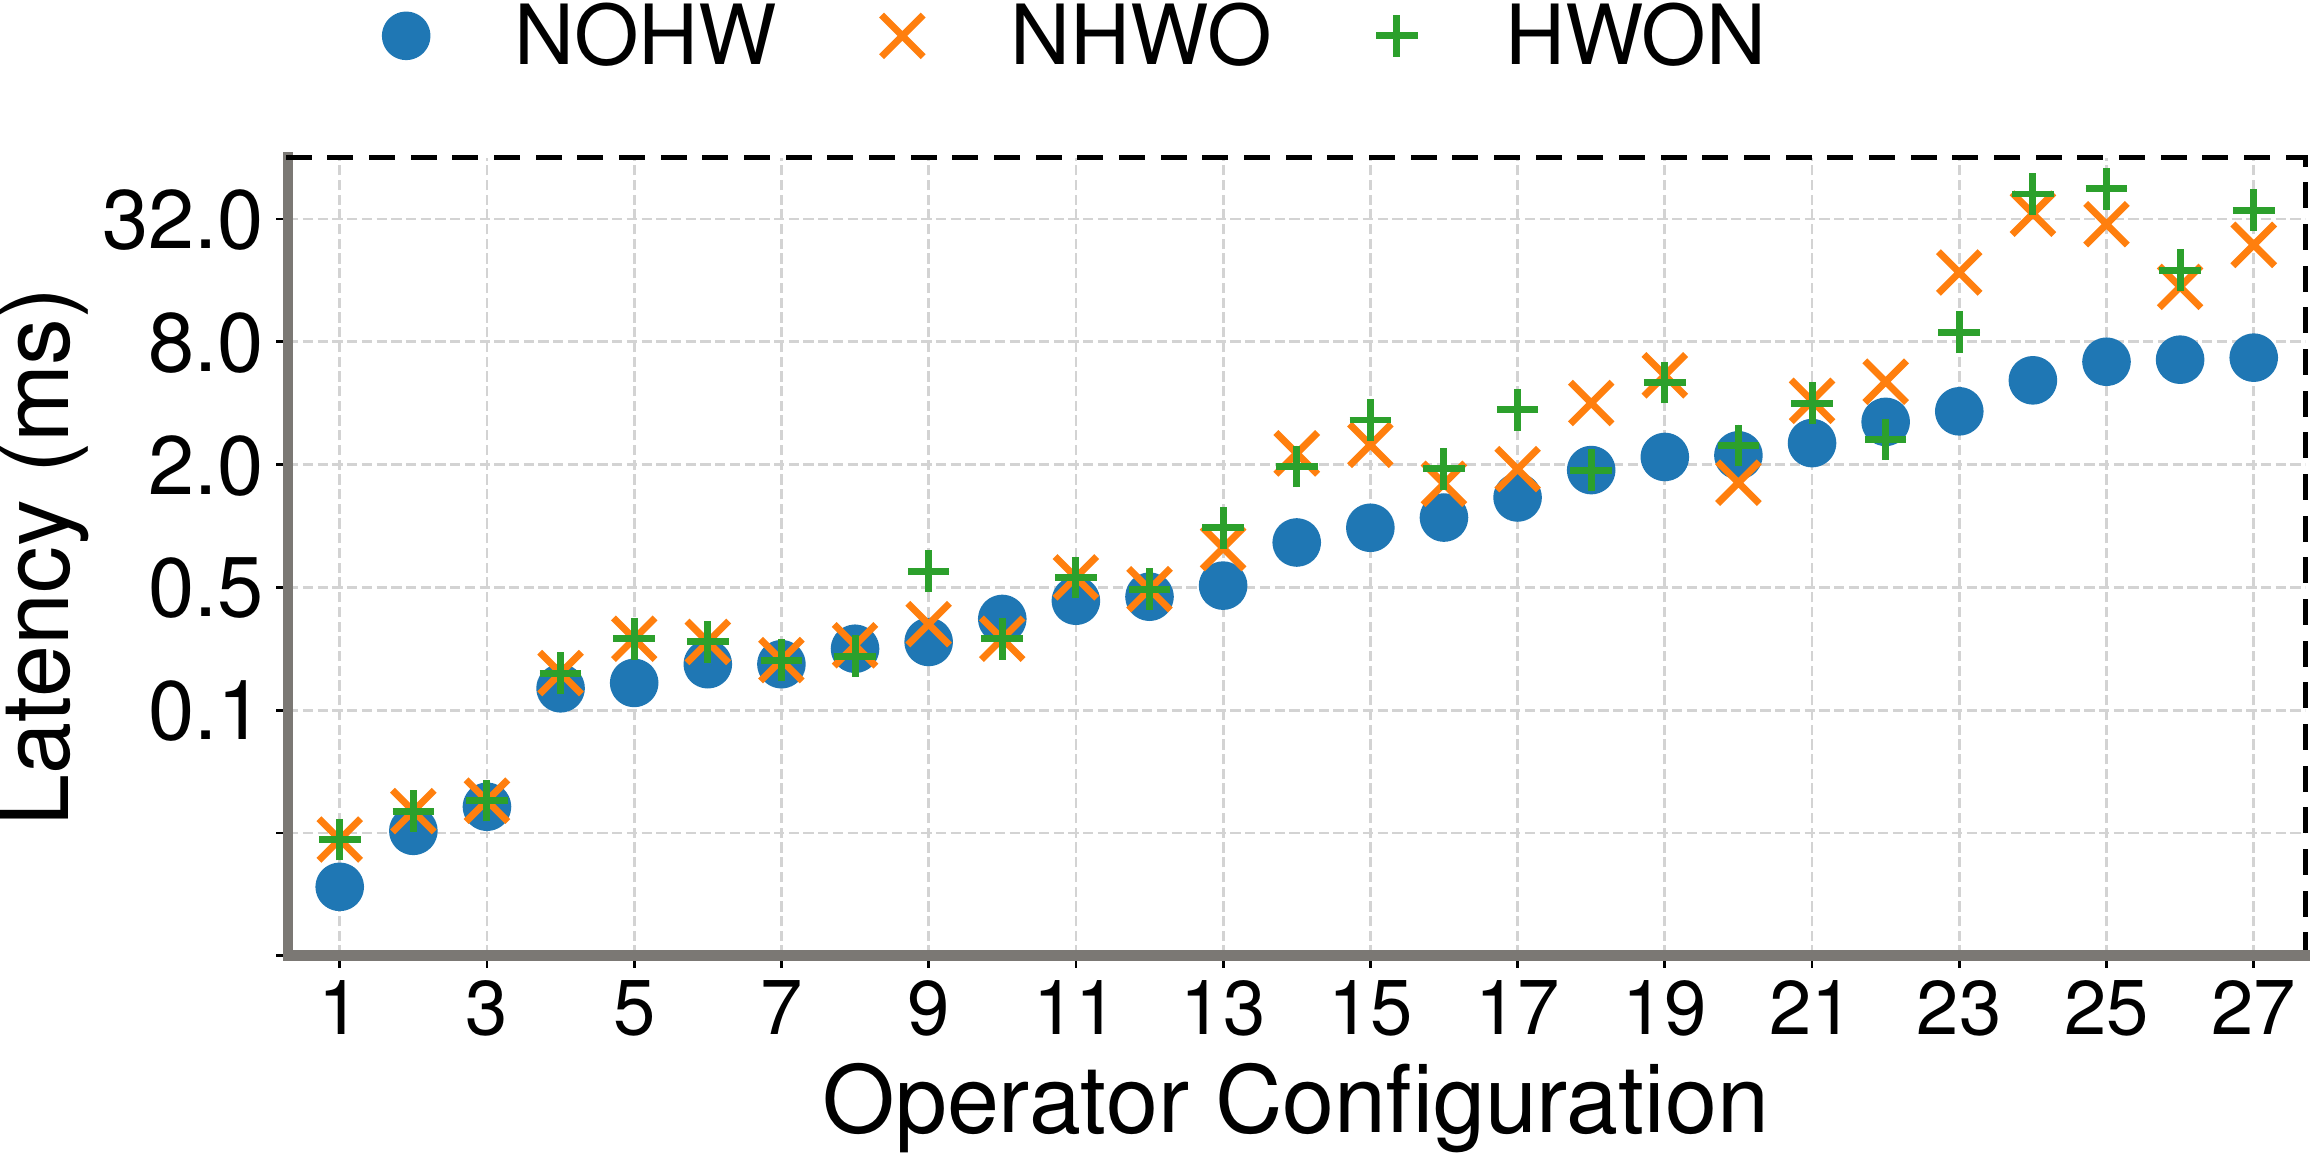}}}\hfill
~
\subfigure[C2D on ARM CPU.]{\label{fig:motiv_C2D_android}{\includegraphics[width=0.32\textwidth]{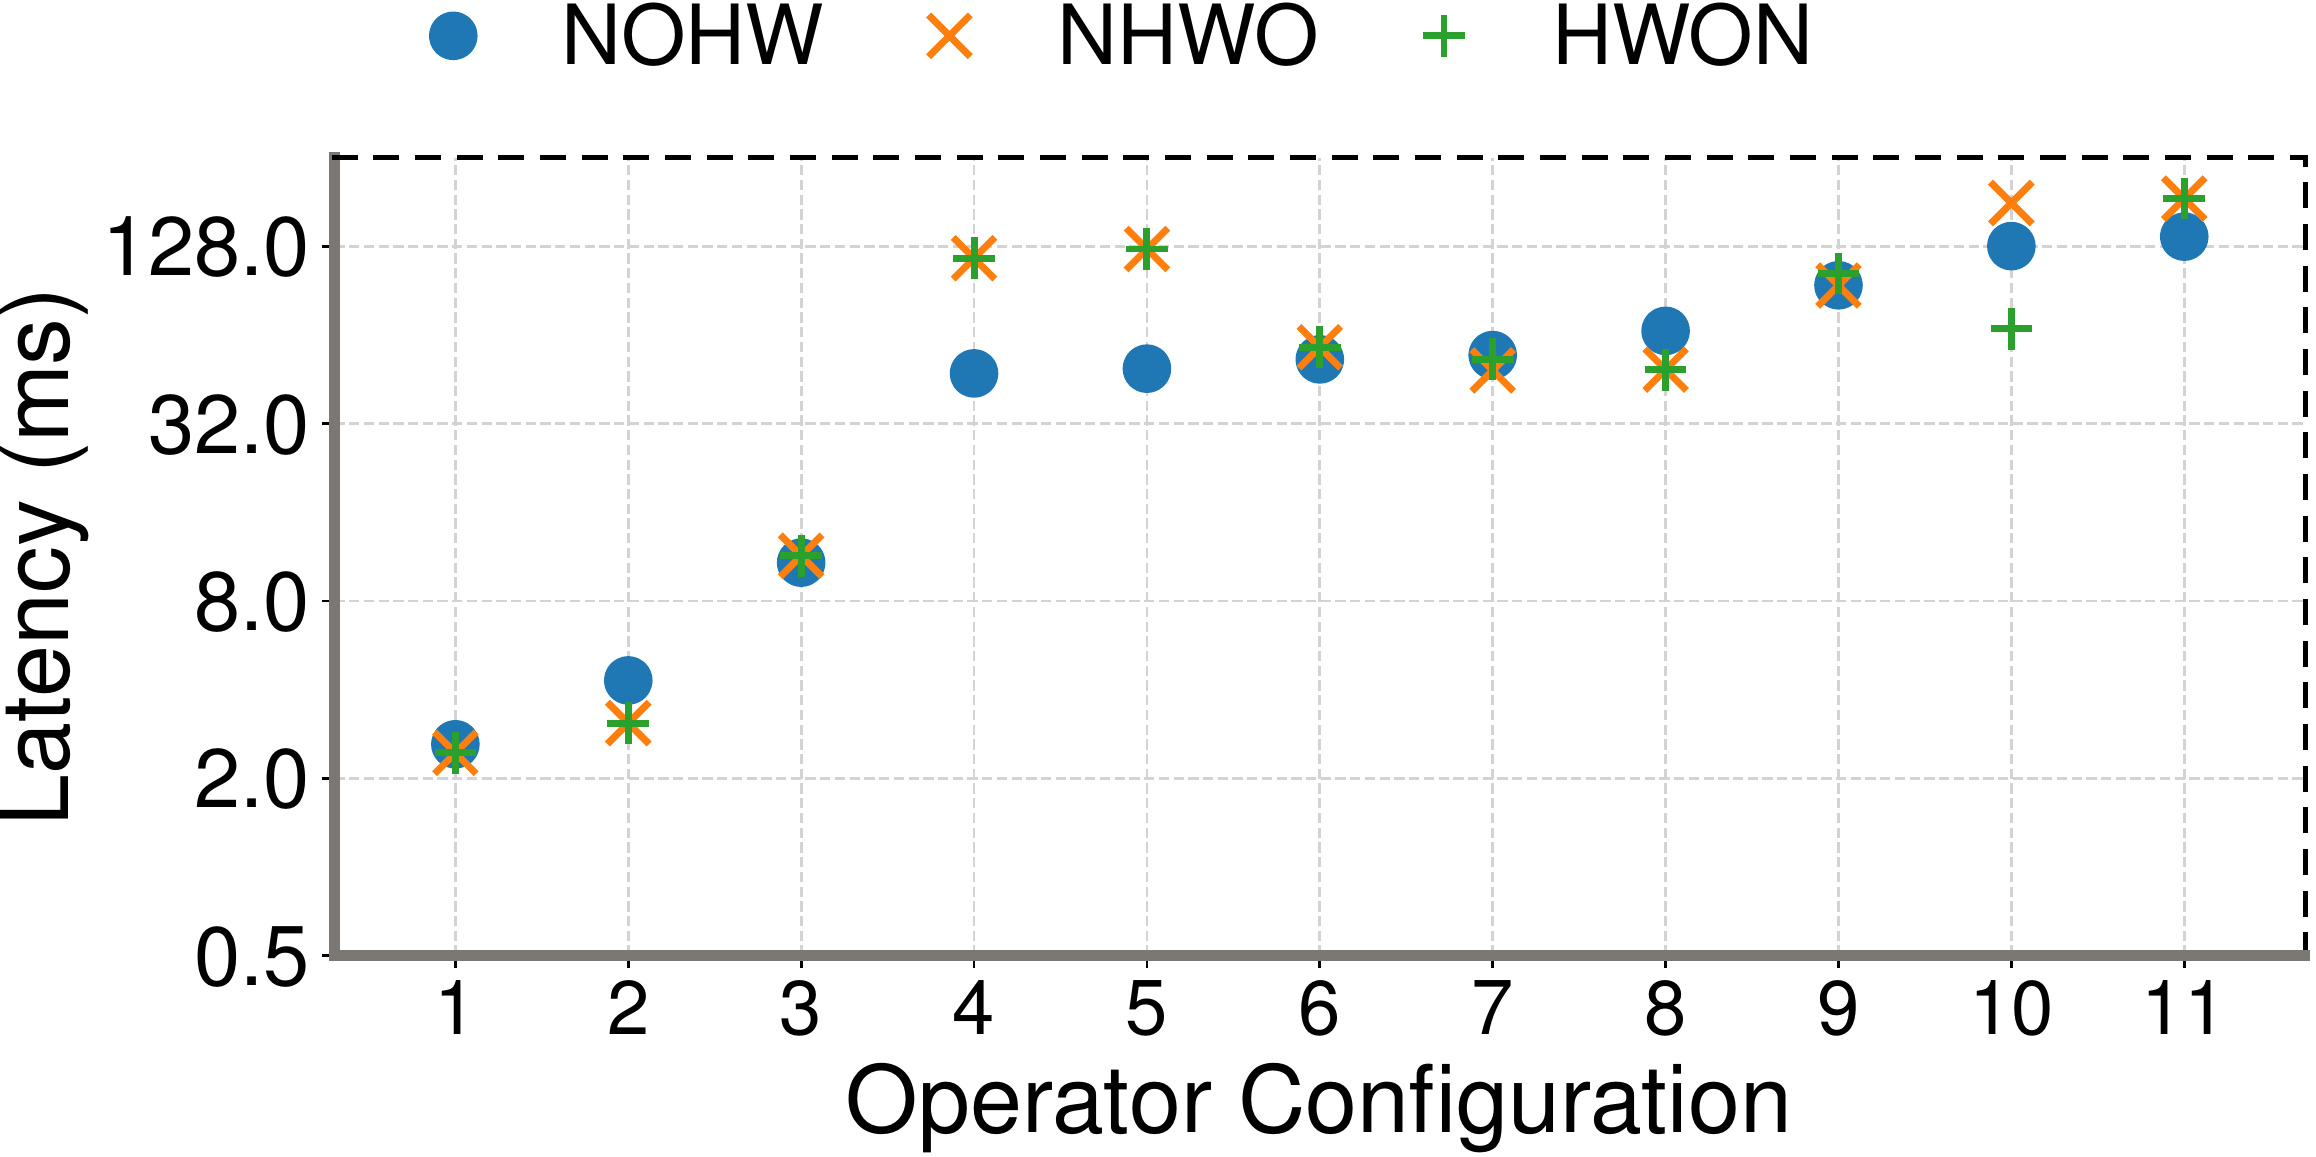}}}\hfill
% \vspace{-0.15in}
\caption{C2D performance with different data layouts on different hardware platforms.}
\label{fig:motiv_C2D}
\vspace{-0.03in}
\end{figure*}
\subsection{Performance of Popular Layouts}
\label{subsec:apdx_motiv}
We illustrate the performance gaps among several popular layouts for C2D with different configurations on 32-core Intel Xeon Silver 4110 CPU@2.10GHz
%(128GB RAM)
, NVIDIA RTX 2080Ti GPU% (CUDA v10.1)
, and Kirin 990 ARM SoC. % (8GB RAM).

\cref{fig:motiv_C2D} shows the results where the latency is in log scale, $N,\, I,\, H,\, W$ represent the batch size, number of input channels, input tensor height, and input tensor width, respectively.
Among different data layouts, $NIHW$ is often used on GPU, $NHWI$ is the default layout on CPU in TensorFlow \cite{abadi2016tensorflow}, while $HWIN$ has been used in digital signal processing \cite{zhang2019tensor}. 
%
%Actually, there also exist attempts for other layouts, such as $IHWN, NIHW[x]$ \cite{liu2019optimizing}, etc. 
%In \cref{fig:motiv_C2D}, we set the kernel layout as $OIhw$, where $O, h, w$ represent the number of filters, the kernel height and the kernel width respectively. 
We adjusted the data and kernel scale, such as the number of channels and feature map size, to generate different tensor configurations. 
%
%Note that there is no difference between $NIHW$ and $IHWN$ when $N=1$, thus some layouts have the same latency. 
%
We observe that the performance of these layouts not only depends on the hardware platform, but also be sensitive to configurations. 
In most cases, $NIHW$ outperforms $NHWI$ and $HWIN$ on NVIDIA GPU. 
However, on Intel CPU and ARM CPU, $NHWI$ and $HWIN$ often perform better than $NIHW$ when the number of input channels is not too large. 
This is because the optimized loop nest of $C2D$ with $NHWI$ on CPU often broadcasts an input value to compute multiple output channels with vector instructions to hide the loads for the input tensor.
In this case, the number of writes on a single memory cell of the output tensor becomes the bottleneck, as it grows with the number of input channels.
%is equal to the number of input channels which gradually turns to the bottleneck when growing. 
%
%It also shows that the best layout could improve the performance by 55.9\%, 87.2\%, and 48.8\% on average on Intel CPU, NVIDIA GPU, and ARM CPU, respectively.

The results in \cref{fig:motiv_C2D} indicate that the best layout could improve the performance by 55.9\%, 87.2\%, and 48.8\% on average on Intel CPU, NVIDIA GPU, and ARM CPU, respectively.
And, it is hard to predict the performance of a specific layout.
In addition, manually exploring different layouts requires much experience and enormous number of trials \cite{barham2019machine}. 
This problem is further exacerbated by the nature of deep learning: the data concerned are multidimensional tensors and a deep model consists of many tensors. 

\subsection{Pad and Store\_at Primitives}
\textbf{pad:} Since deep learning models are often deployed on GPU, we introduce another primitive to address layout optimization on such many-core architectures. Take NVIDIA GPU as an example, 
threads can access data from global memory (off-chip DRAM) or shared memory (on-chip memory, shared inside a thread block). 
since accessing off-chip global memory can consume up to thousands of cycles, 
shared memory access scheduling is vital to performance optimization.
On the other hand, fetching data to shared memory first, can also help to achieve memory coalescing for global memory (\textit{e.g.}, carrying 128 bytes for each transfer to fill up the bandwidth). 
Moreover, shared memory 
which is then organized with interleaving banks to improve the throughput. 
However, bank conflicts arise when different threads access distinct memory locations but in the same bank simultaneously. % and cause serial transfers. 

To avoid this, we pad the data so that memory requests from a half-warp of threads are distributed into distinctive banks:
because the scheduler can gather multiple threads to fetch the data simultaneously as there is no thread divergence at this without-computation stage.

We develop a pad primitive to cover this technique.
\mint{python}|pad(tensor, dimension, pad_size)|
This primitive appends zeros at the end of the selected dimension. If the original dimension size is $N$, it will expand to a new size of $(N+pad\_size)$. 
%Note that although we target this primitive on tensors in shared memory, it can also be applied on general tensors. 
%For example, given a tensor $A$ with shape $M\times N$, then applying \mintinline{python}{pad(A, 1, 1)} will attach a redundant element to the second dimension of A resulting a new shape $M \times (N + 1)$. 

The index transformation for pad is an identity mapping:
\begin{align*}
	A[i] \mapsto A[i] \, .
% 	\label{eq:pad_index_transform}
\end{align*}

\textbf{store\_at:} In some cases, there are multiple constant tensors in an operator. For example, a fully connected layer has a constant weight tensor $W$ with shape of $K \times M$ and a constant bias tensor $b$ of length $M$. Whenever a column of $W$ is multiplied with the input, an element of $b$ will be added to the result. We can fuse them by attaching each element of $b$ to the corresponding column of $W$ to generate a new tensor with shape of $(K + 1) \times M$. Through another transposition to $M \times (K + 1)$, we may compute the matrix multiplication and bias addition together with less memory loads and better locality. Such fusion is analogous to the transformation between \emph{Array of Structure} (AoS) and \emph{Structure of Array} (SoA) in traditional compilers \cite{sung2012dl, tseng2014automatic, majeti2016automatic, kronawitter2018automatic}. We develop a store\_at primitive which attaches tensor $S$ to tensor $T$, at the given $dimension$:
\mint{python}|store_at(S, T, dimension)|
This primitive requires the shapes of $S$ and $T$ are differed in only one dimension. 
%For example, if $S$ has a shape $N$ while $T$ is of $M \times K \times N$, the attachment will fail. Otherwise, this will produce $M\times(K+1)\times N$, an aggressive data expansion. However, a fuse primitive can be applied to $M, K$ first, then another store\_at can generate a new shape $(MK + 1)\times N$. The $dimension$ parameter is only useful when there are multiple possible positions to attach.
Suppose $T$ has a shape of $M \times N$, and $S$ has a shape of $N$, then the index transformation is
\begin{align*}
	S[i] \mapsto T[M][i] \\
	T[j][k] \mapsto T[j][k]\, .
\end{align*}

Automation for these two primitives is similar to unfold, although we do not include them in \cref{sec:automation}. For instance, we can deploy an actor to decide whether to pad a tensor. And the padding dimension parameter can always be the last dimension of a tensor and the pad size can always be 1.
% Formally, we summarize the advanced primitives in \cref{tab:adv_layout_prims}:
% \begin{table*}
% 	\centering
% 	\small
% 	\caption{Advanced layout primitives.}
% 	\label{tab:adv_layout_prims}
% 	\begin{tabular}{cccc}
% 		\toprule
% 		\textbf{Primitive} &\textbf{Facility} &\textbf{Parameter} & \textbf{Index Transformation}\\
% 		\midrule
% 		unfold & tile a dimension with overlap & dimension $I$, block size $B$, stride $S$ & $A[Ki + r] \mapsto A^\prime[\frac{i}{\floor{\frac{B-W}{K}} + 1}][Ki + r - \frac{Si}{\floor{\frac{B-W}{K}} + 1}]$\\
% 		\midrule
% 		pad & pad a dimension with zeros & dimension $I$, pad size $p$ & $A[i] \mapsto A^\prime[i]$\\
% 		\midrule
% 		store\_at & attach a tensor to another & source and target $S, T$, attach dimension $I$ & $S[i]\mapsto T^\prime[M][i]; \quad		T[j][k] \mapsto T^\prime[j][k]$ \\
% 		\bottomrule
% 	\end{tabular}
% \end{table*}

\subsection{Features for Cost Model}

The extracted features mainly consist of 5 parts: computation, loop structure, GPU threads, accessing expression, and compilation annotations.

The computation we considered includes float-point or fixed-point multiplication, addition, subtraction, division, modulo, and logical operations:
\begin{enumerate}
    \item The total count of each type of computation;
    \item The count of each type of computation inside each loop.
\end{enumerate}

The loop structure features involve the depths in the loop nest and the trip counts for all loops. To guarantee a fixed length for the extracted feature, we limit the maximum number of loops to 32.

Afterwards, GPU threads related features record the attaching loop depth for $blockIdx.x$, $blockIdx.y$, $blockIdx.z$, $threadIdx.x$, $threadIdx.y$, $threadIdx.z$, and their extents.

The tensor accessing expression features include storage scope, accessing type, accessing count, tensor size, and strides for each loop iterator:
\begin{enumerate}
    \item The storage scope is classified into three categories: \emph{general}, \emph{local} and \emph{shared}. As the name indicates, local scope refers local arrays, shared scope denotes tensor in shared memory and others belong to the general scope;
    \item Accessing type is either \emph{read} or \emph{write}. Note that in a statement, the same tensor can have different accessing types. For example, given $C = C + A * B$, we treat the left $C$ and the right $C$ as write access and read access respectively;
    \item Tensor size is nothing but the storage size of each tensor;
    \item As to the strides for each loop iterator, we illustrate this through an example. Given an expression $A[2i][j]$, the stride for iterator $i$ is 2 while the stride for $j$ is 1. If a iterator shows several times in the expression, we only extract the stride for its last appearance.
\end{enumerate}
Similar to loop structures, we set the maximum number of accesses recorded as 8 to get a fixed length of features.

The last part includes compilation annotations. Specifically, we record the annotation position (annotating on which loop) for \emph{unroll}, \emph{parallel}, and \emph{vectorize} respectively, and the annotation value for \emph{unroll} (the maximum unroll depth). 
